# Supplementary material for: Learning Control Policies for Fall prevention and safety in bipedal locomotion
Source: arXiv:2201.01361 source file (2022-01-04)
Supplement: Supplementary file 1 [file appendix.tex]

% The environment used here (theappendices) is a wrapper for the basic appendices environment which changes the appearance of the title page and the structure and appearance of the appendices in the table of contents and PDF bookmarks. The original functionality can be restored by simply removing the 'the' from the \begin{} and \end{} statements below.

\begin{theappendices}

\chapter{Experimental Equipment}
A telescope and a spectrometer were used to analyze the sun. Many other instruments were used.

\chapter{Data Processing}
Data was processed before being added to this document.

\end{theappendices}
